# Supplementary material for: RVI-SAC: Average Reward Off-Policy Deep Reinforcement Learning
Source: arXiv:2408.01972 source file (2024-08-04)
Supplement: Supplementary file 2 [file additional_results.tex]

\section{Additional Results}

\subsection{Average reward evaluation}
\label{sec:appendix_average_reward_evaluation}

図\ref{fig:average_reward}は，評価値をaverage reward(total\_reward / survival\_step)に設定したときの，RVI-SACと様々な割引率をもつSAC，ARO-DDPGの学習曲線を示しす．
ここで，SwimmerとHalfCheetah環境にはterminationが存在しないため，average rewardで評価した結果とtotal rewardで評価した結果(図\ref{fig:main_result})が同じになる．
この結果は，図\ref{fig:main_result}に示す結果と同様に，RVI-SACがaverage rewardにおいても全体的に高い性能を示していることを示している．
\begin{figure*}[htp]
  \begin{subfigure}{1.0\textwidth}
    \centering
    \includegraphics[scale=0.5]{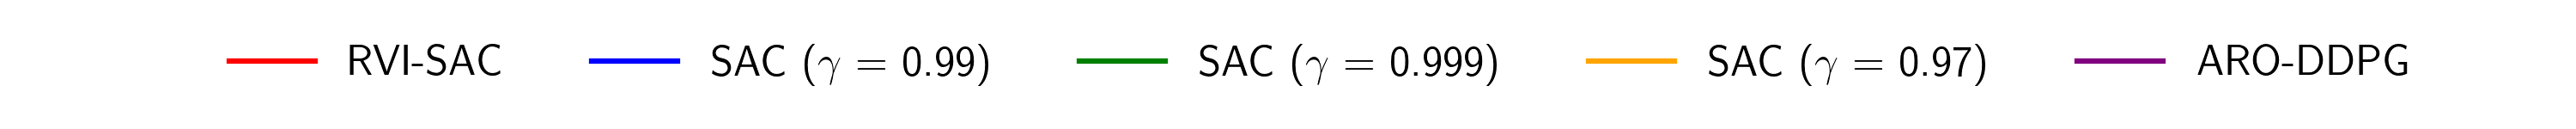}
  \end{subfigure}
  \centering
  \begin{subfigure}{.3\textwidth}
    \centering
    \includegraphics[width=\linewidth]{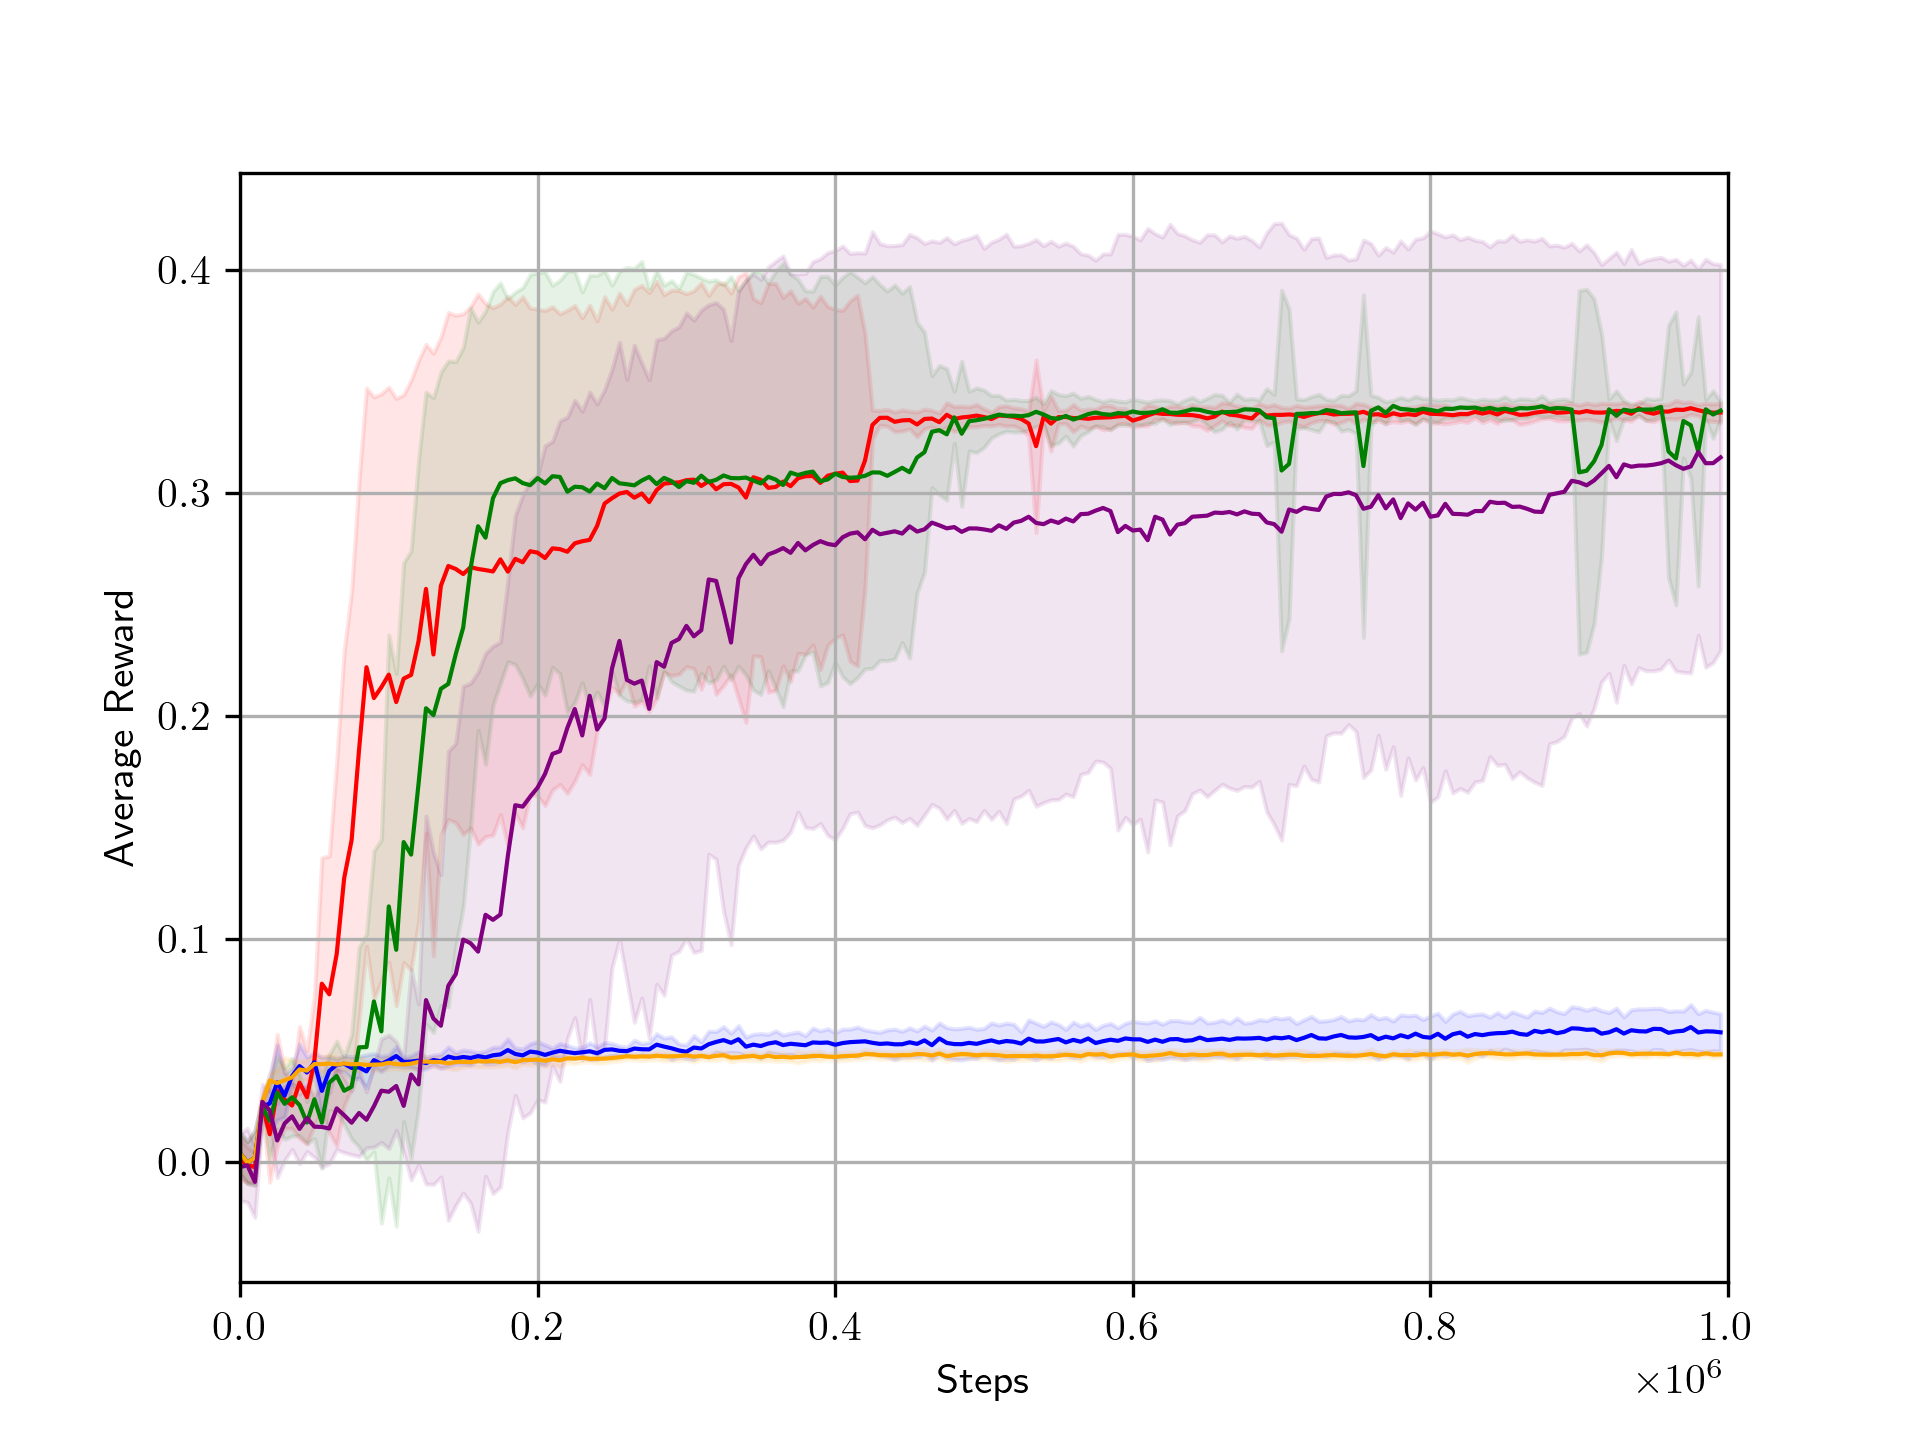}
    \caption{Swimmer}
    \label{fig:average_reward_swimmer}
  \end{subfigure}
  \begin{subfigure}{.3\textwidth}
    \centering
    \includegraphics[width=\linewidth]{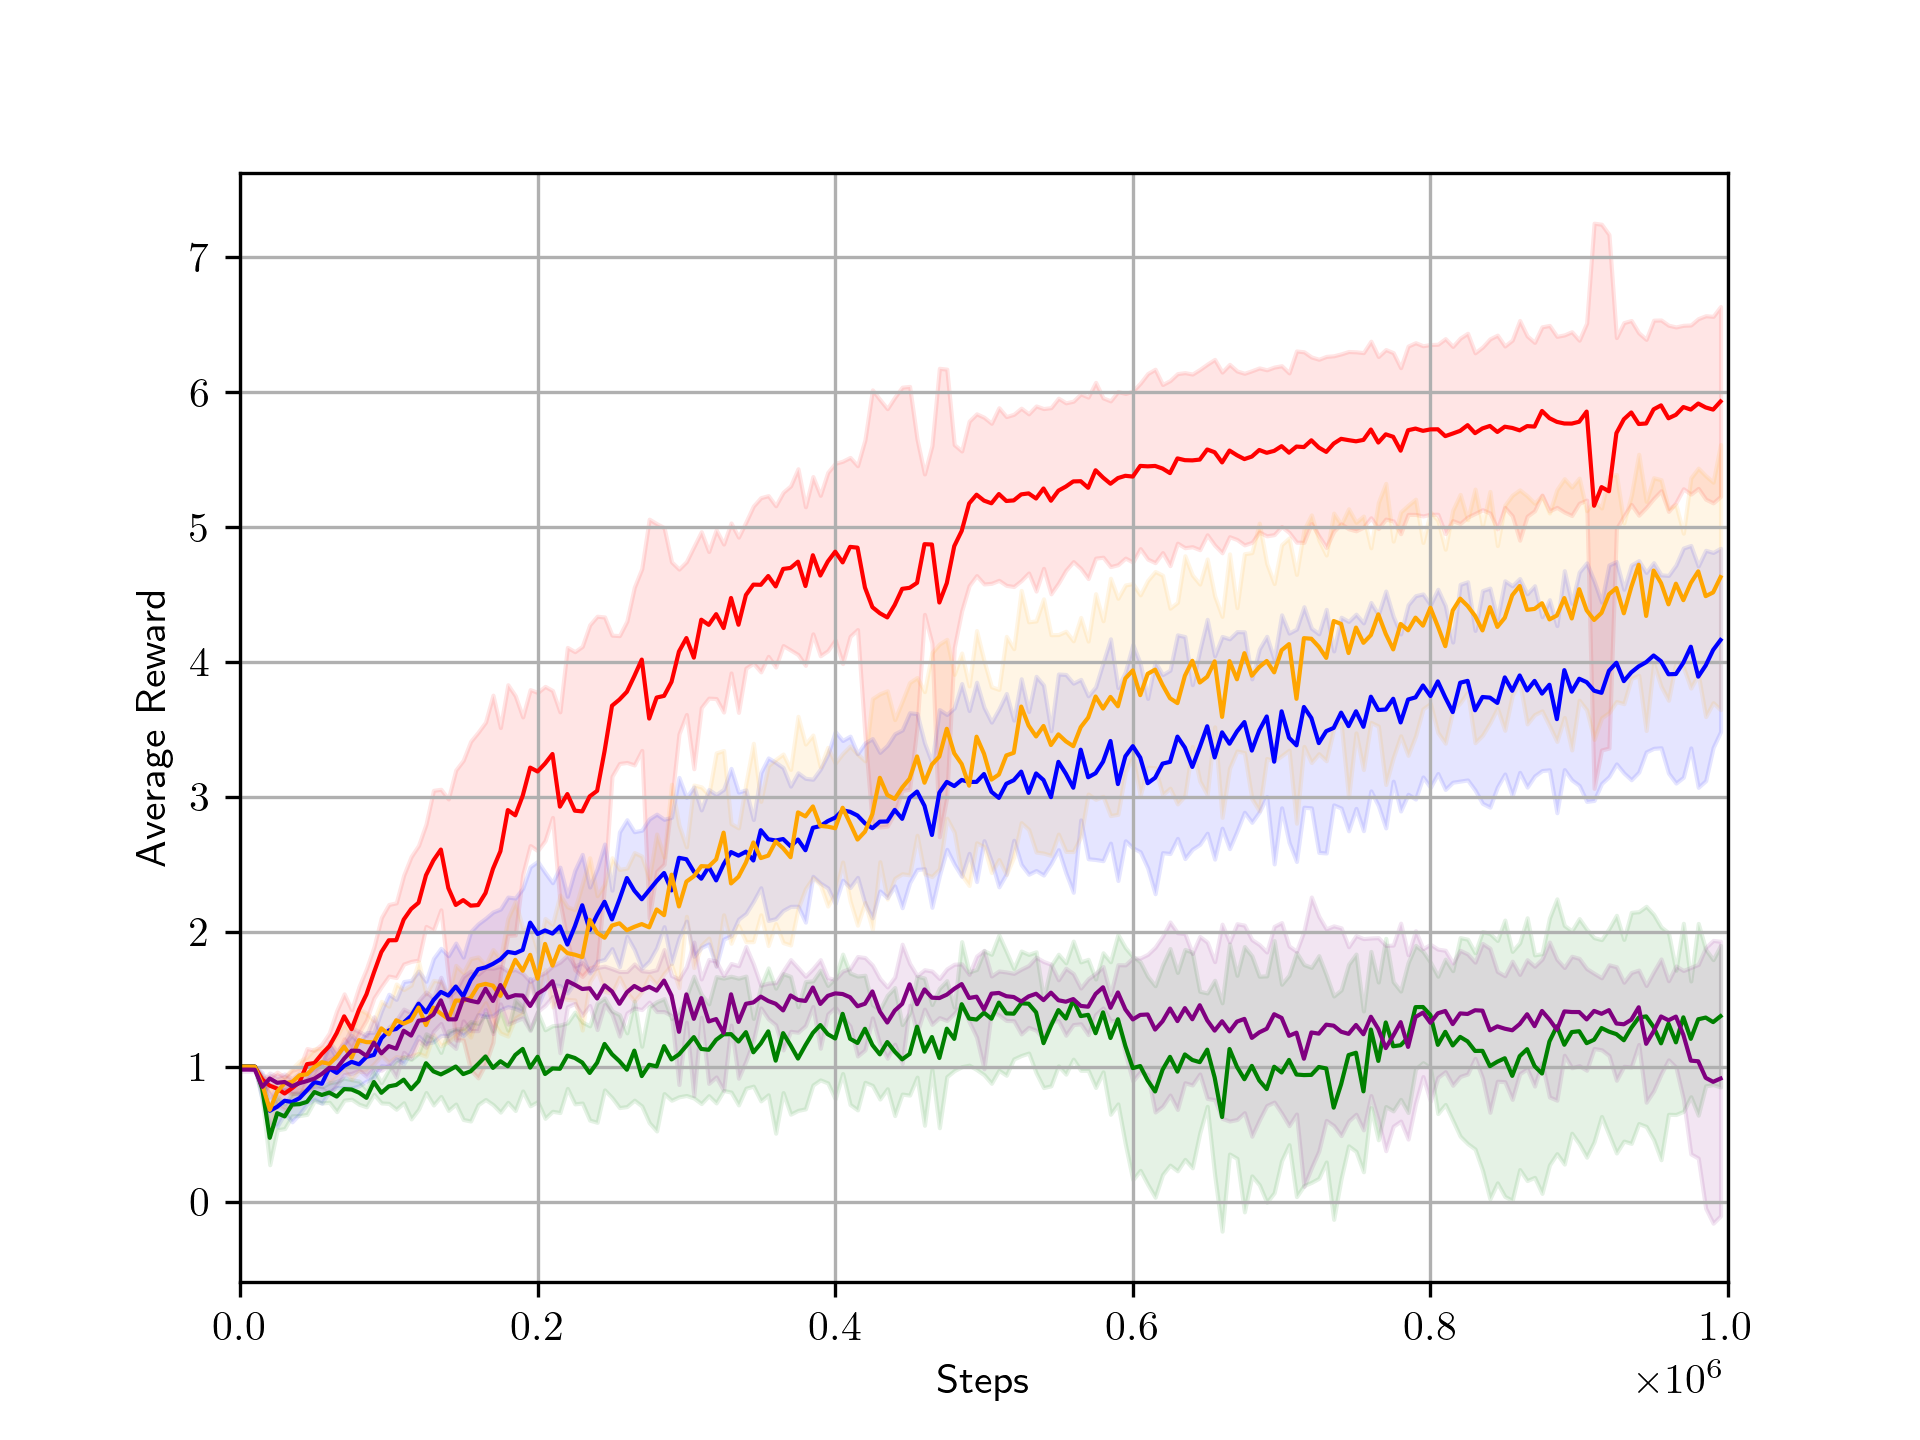}
    \caption{Ant}
    \label{fig:average_reward_ant}
  \end{subfigure}
  \begin{subfigure}{.3\textwidth}
    \centering
    \includegraphics[width=\linewidth]{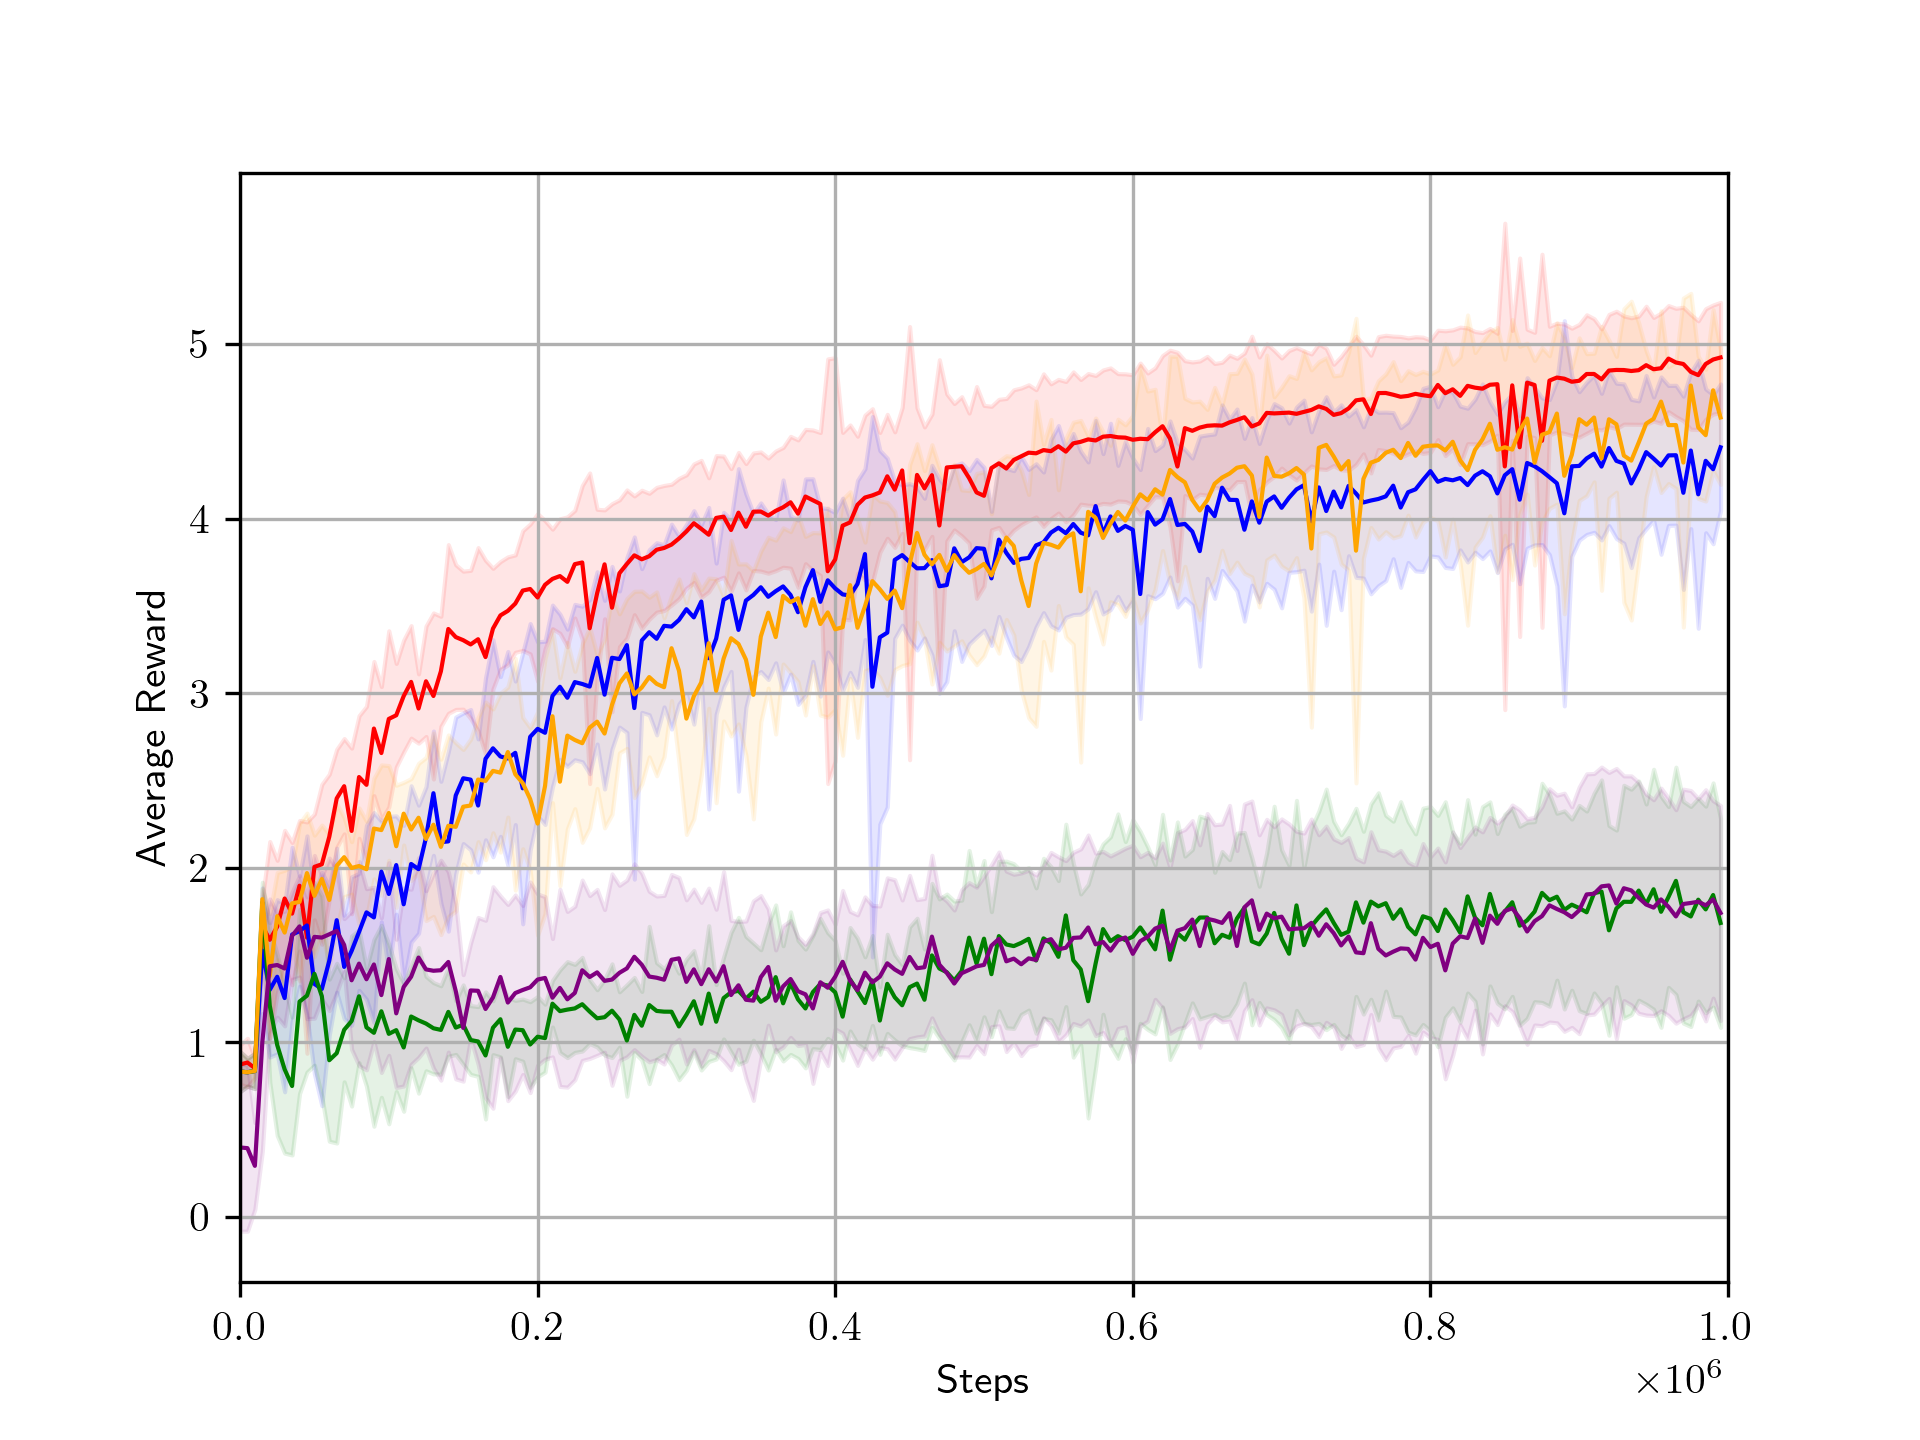}
    \caption{Walker2d}
    \label{fig:average_reward_walker2d}
  \end{subfigure}%

  \begin{subfigure}{.3\textwidth}
    \centering
    \includegraphics[width=\linewidth]{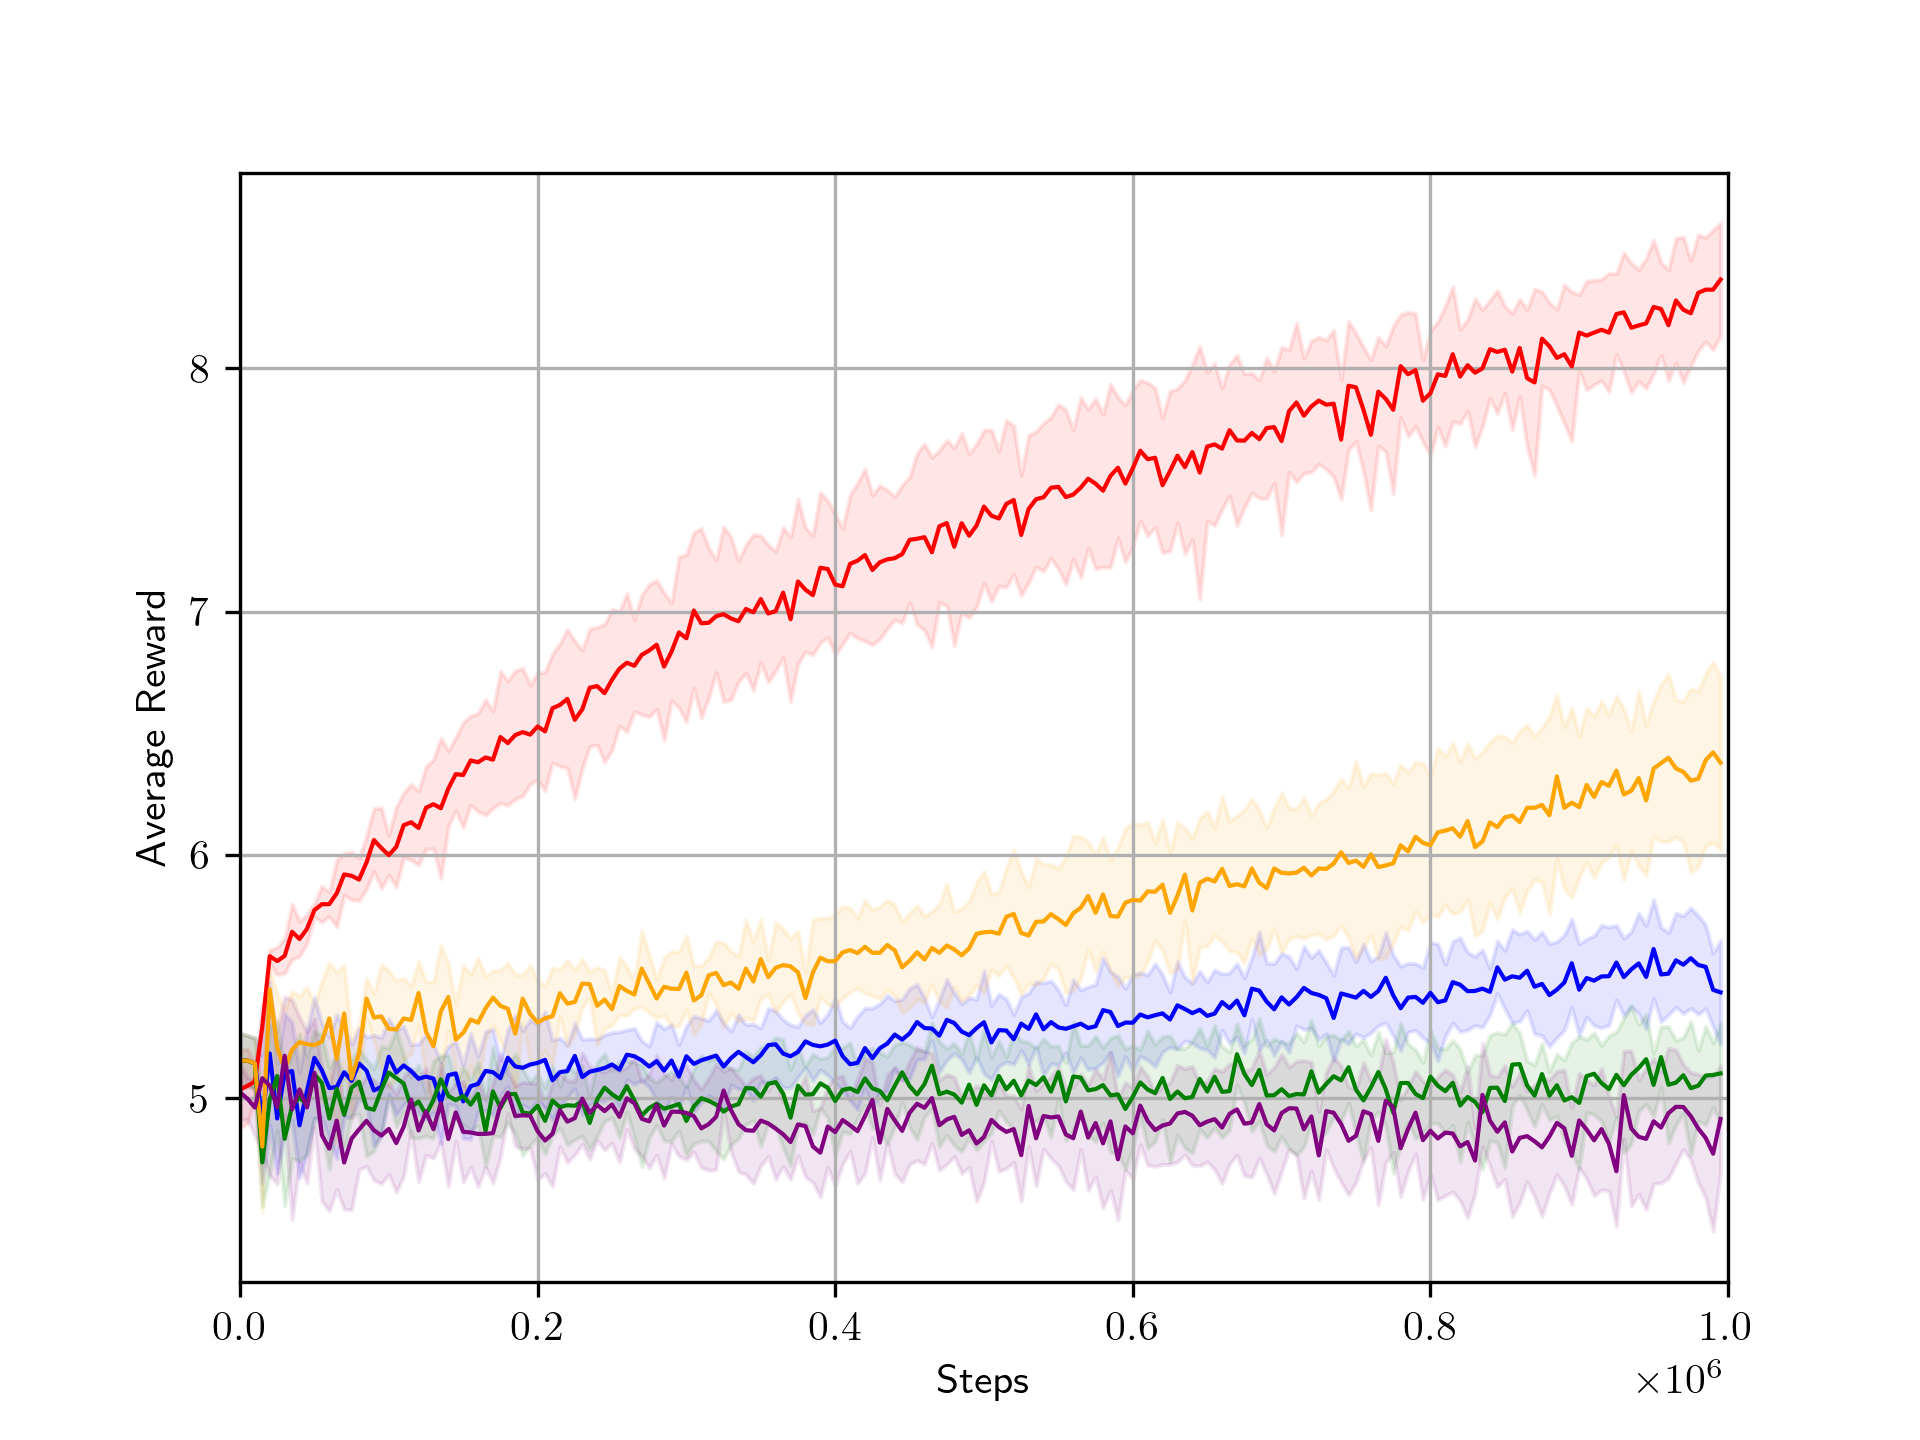}
    \caption{Humanoid}
    \label{fig:average_reward_humanoid}
  \end{subfigure}
  \begin{subfigure}{.3\textwidth}
    \centering
    \includegraphics[width=\linewidth]{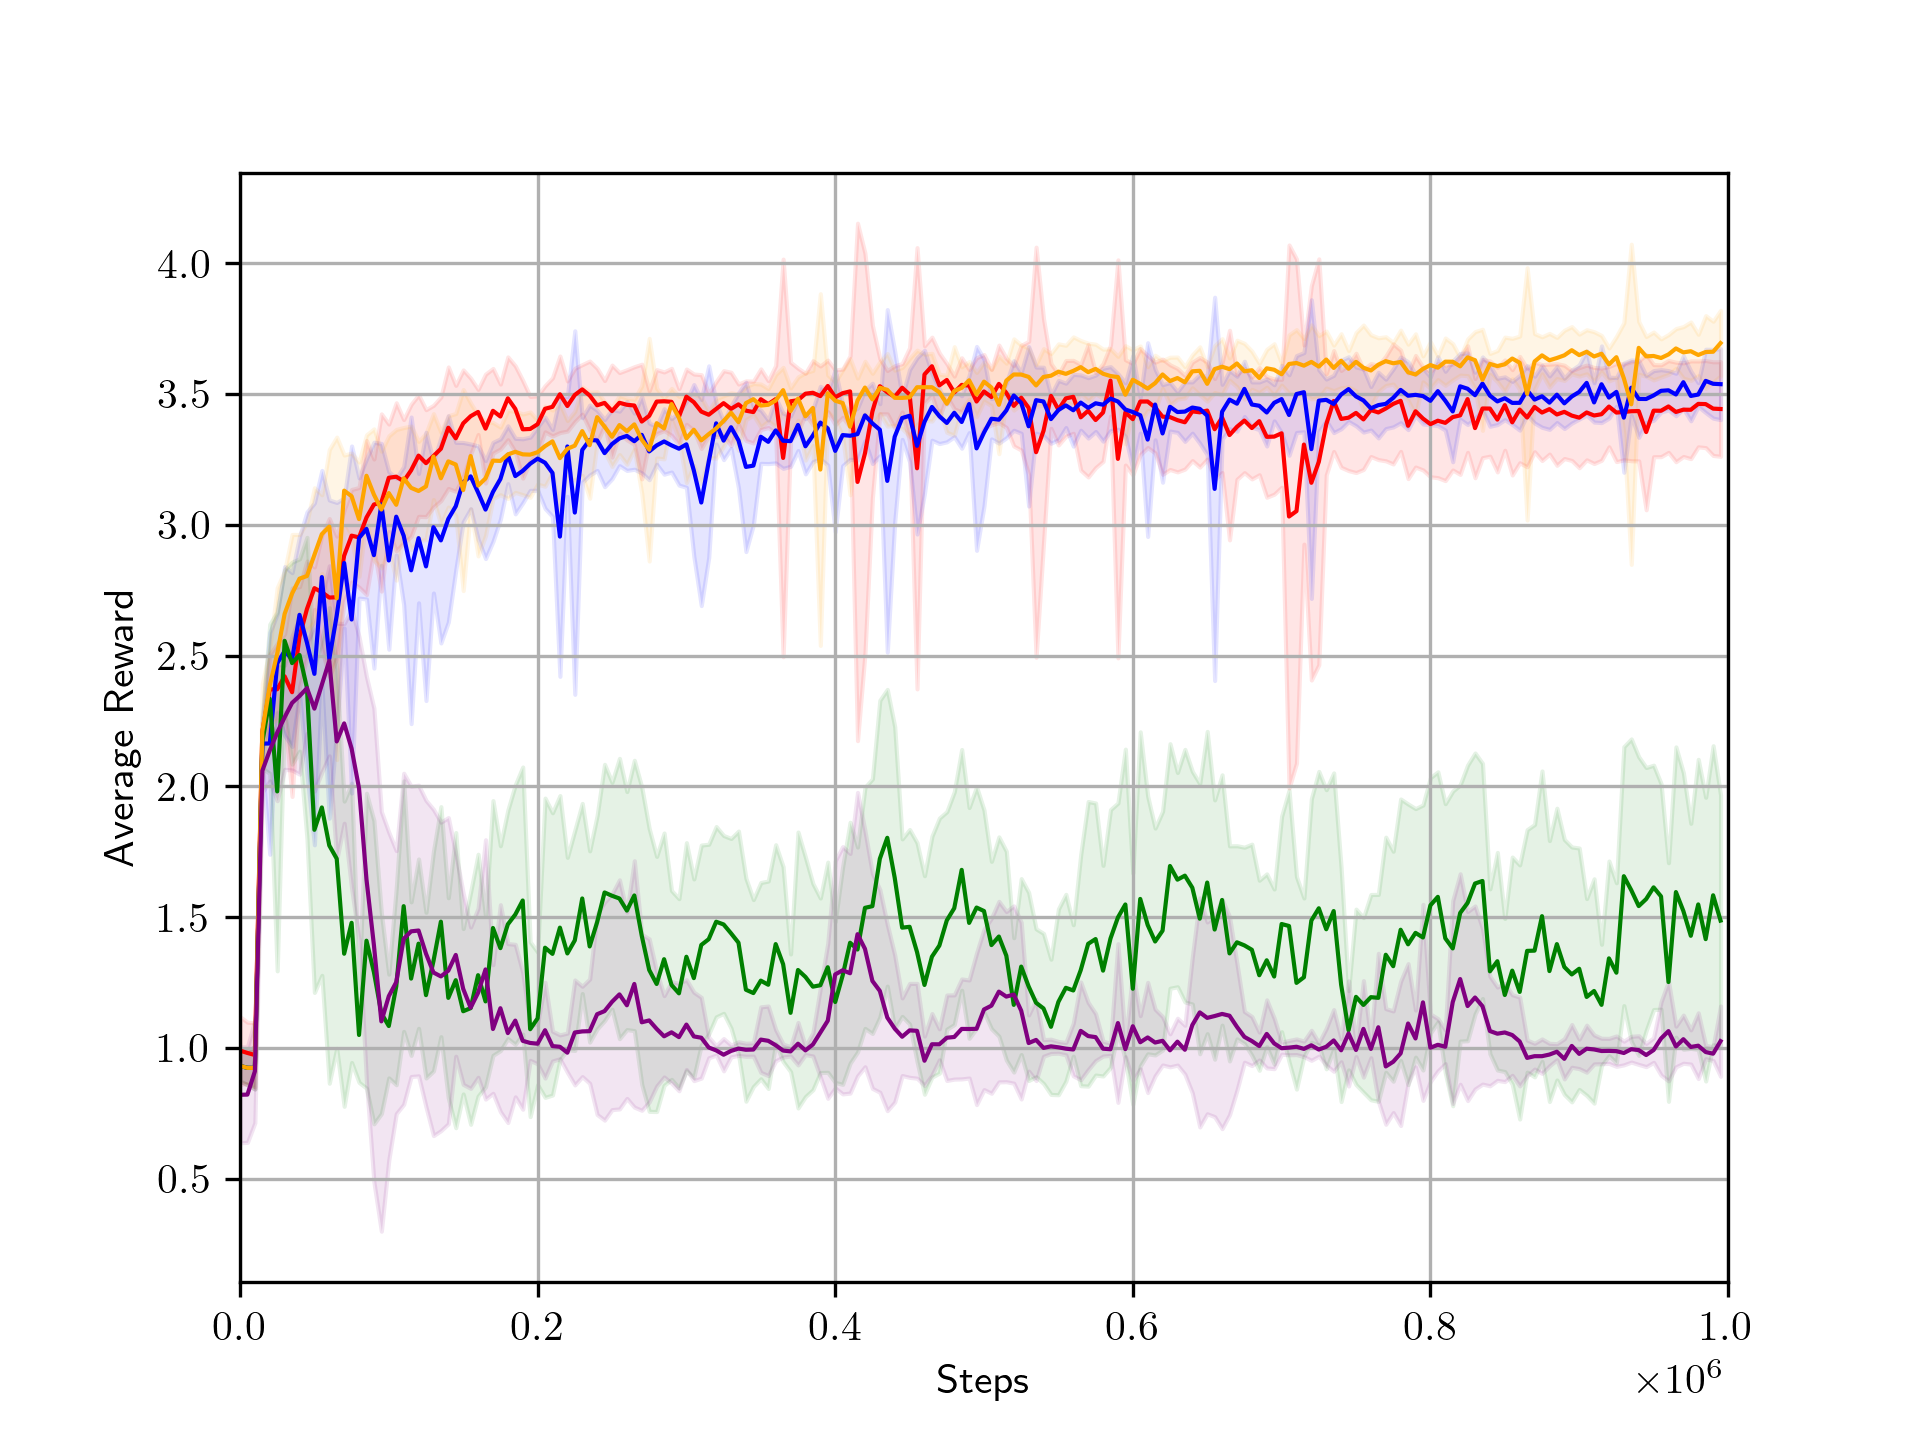}
    \caption{Hopper}
    \label{fig:average_reward_hopper}
  \end{subfigure}
  \begin{subfigure}{.3\textwidth}
    \centering
    \includegraphics[width=\linewidth]{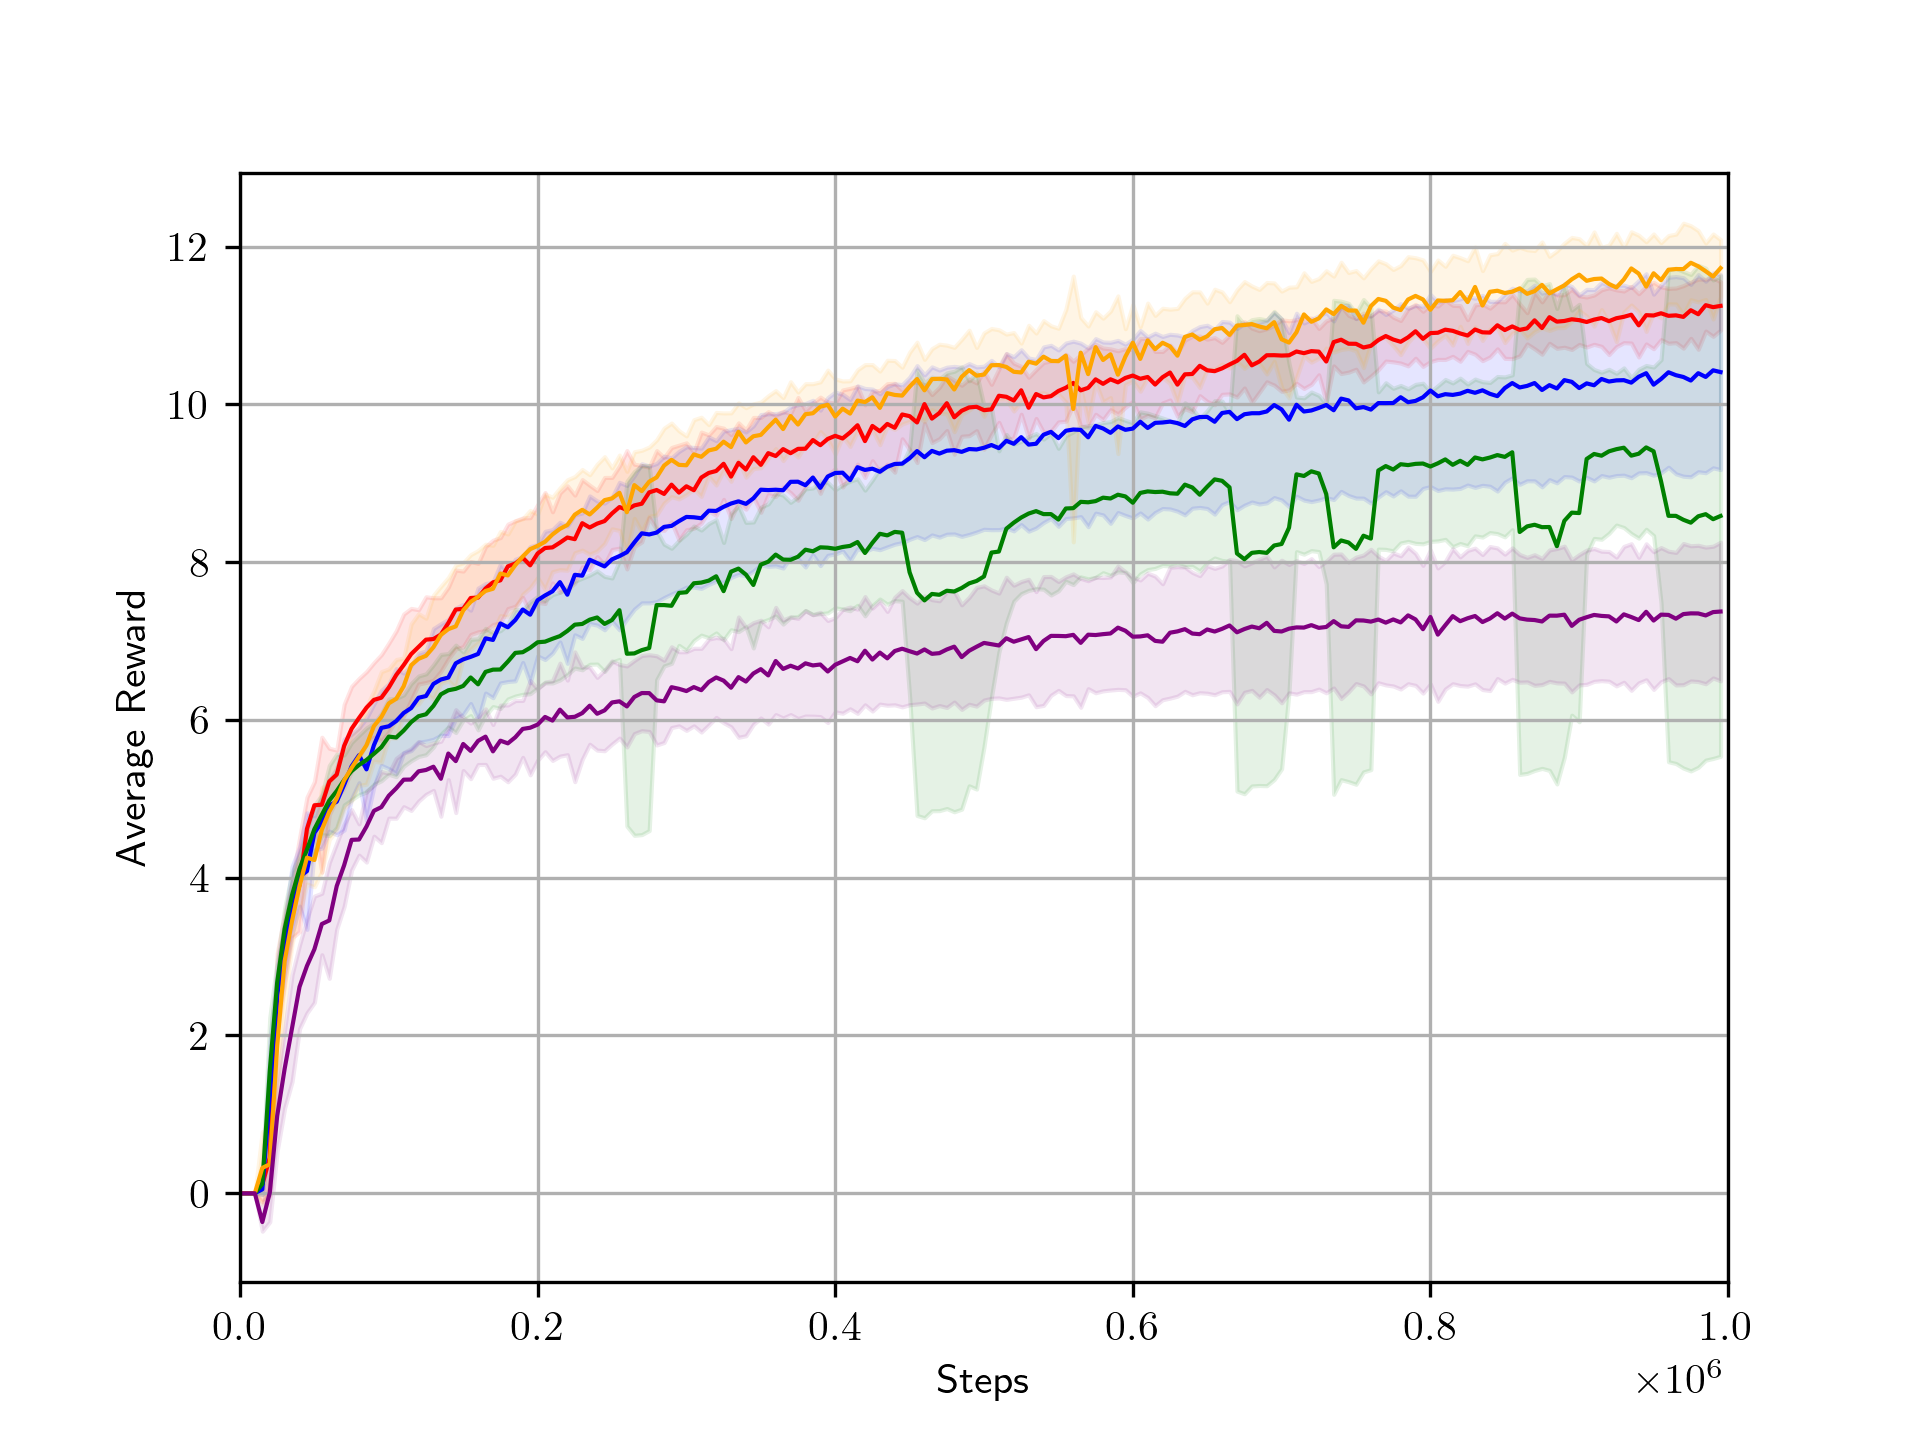}
    \caption{HalfCheetah}
    \label{fig:average_reward_halfcheetah}
  \end{subfigure}
  \caption{Learning curves for the Gymnasium continuous control tasks. The shaded region represents half a standard deviation of the
    average evaluation over 10 trials.}
  \label{fig:average_reward}
\end{figure*}

\subsection{Performance comparison of RVI-SAC and SAC with Reset}
\label{sec:appendix_sac_with_reset}

\begin{figure*}[htp]

  \begin{subfigure}{1.0\textwidth}
    \centering
    \includegraphics[scale=0.6]{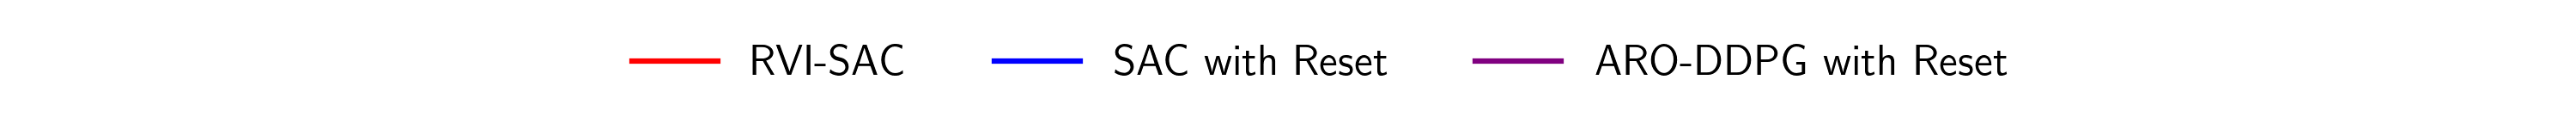}
  \end{subfigure}

  \centering
  \begin{subfigure}{.3\textwidth}
    \centering
    \includegraphics[width=\linewidth]{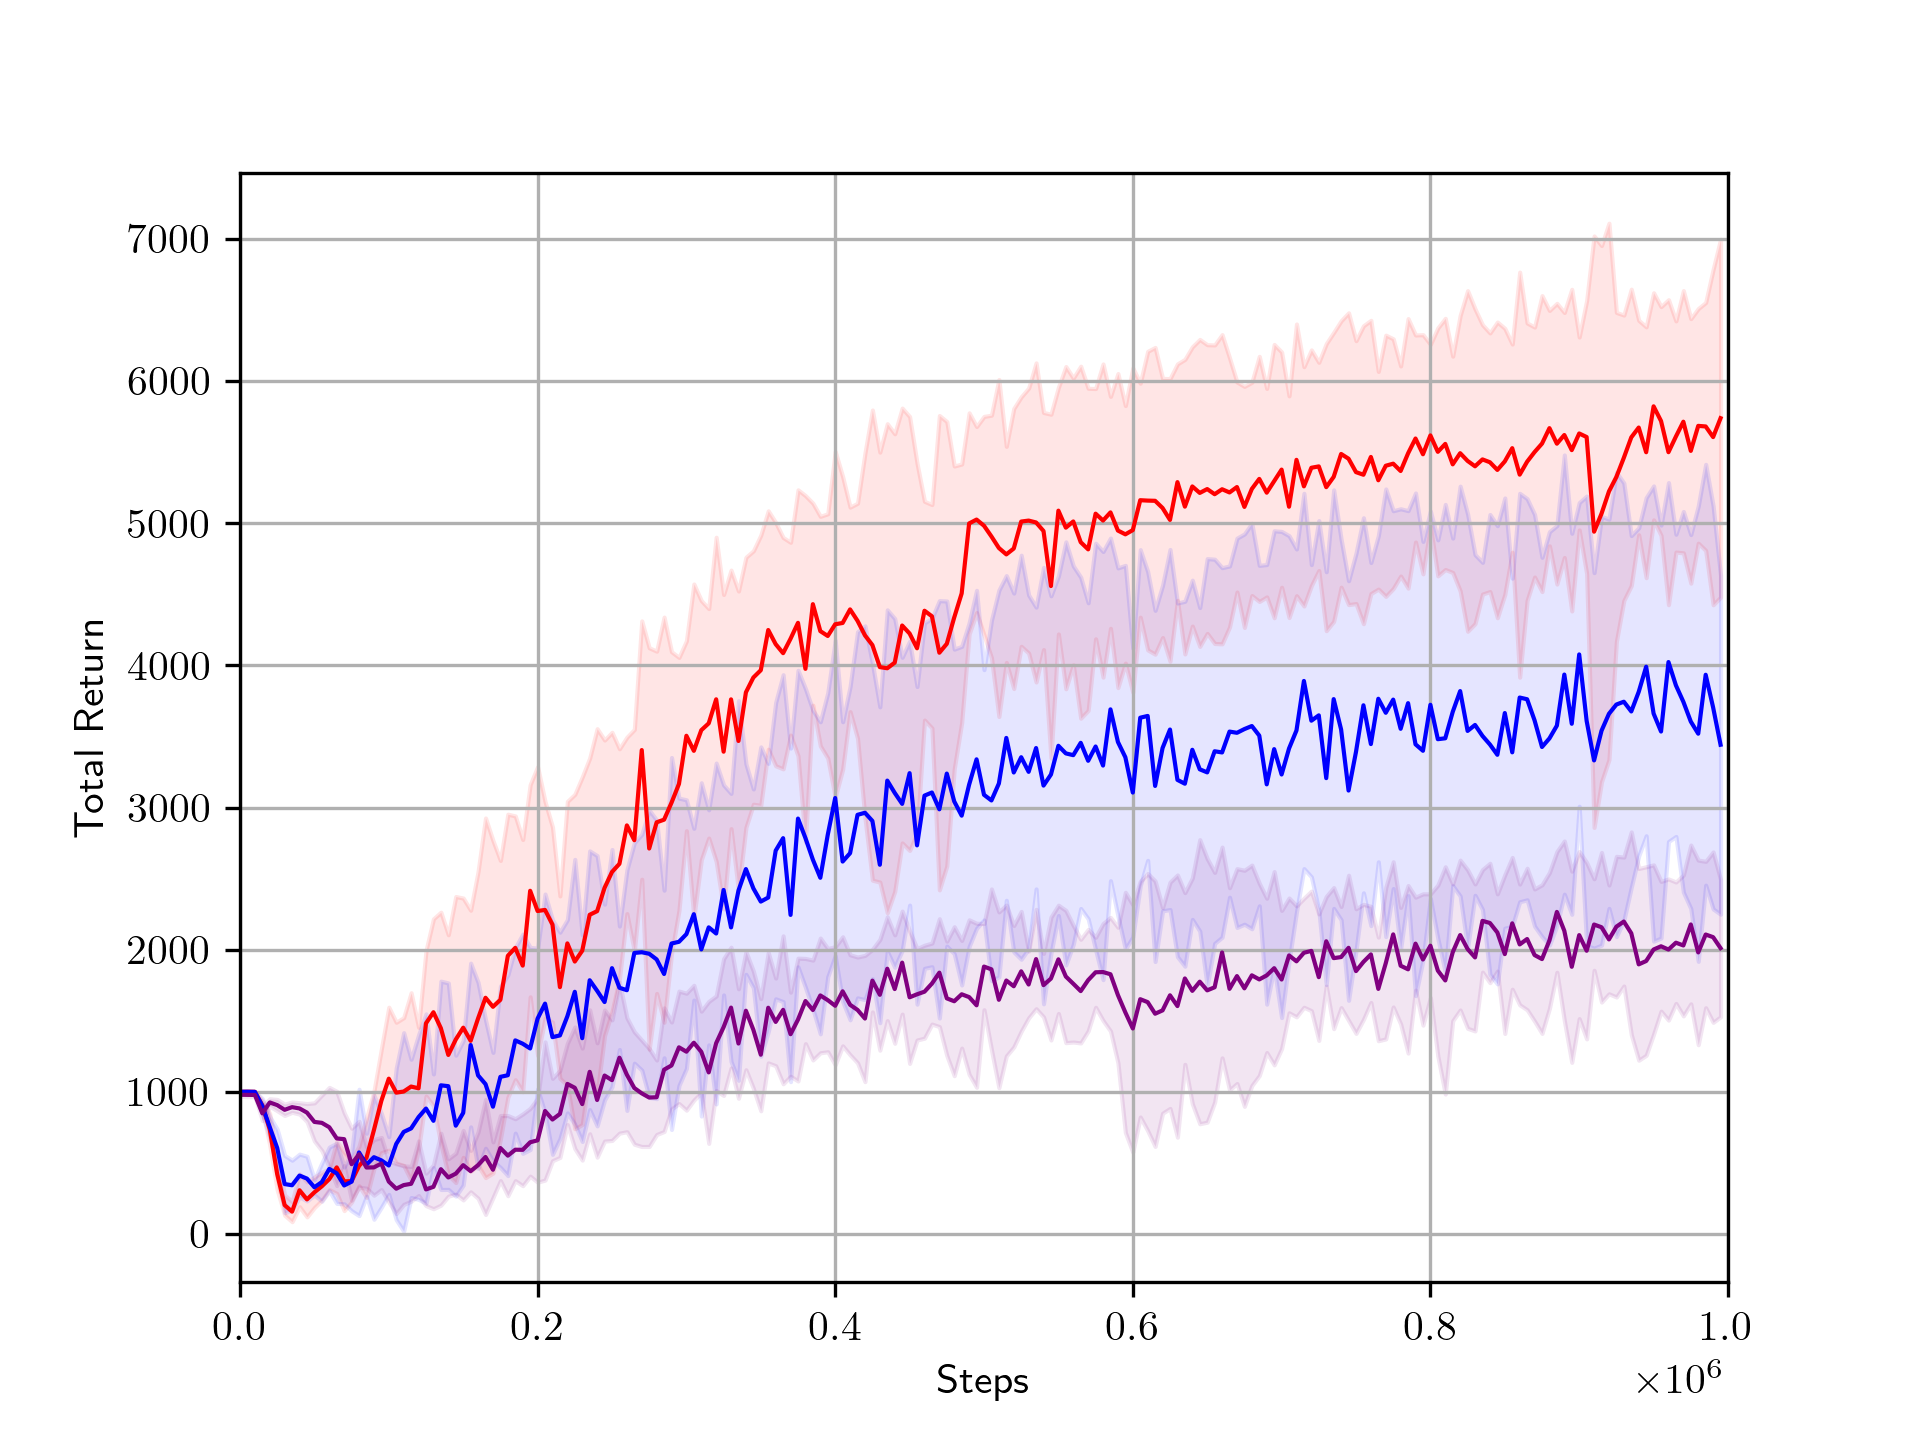}
    \caption{Ant}
    % \label{fig:sac_with_reset}
  \end{subfigure}
  \begin{subfigure}{.3\textwidth}
    \centering
    \includegraphics[width=\linewidth]{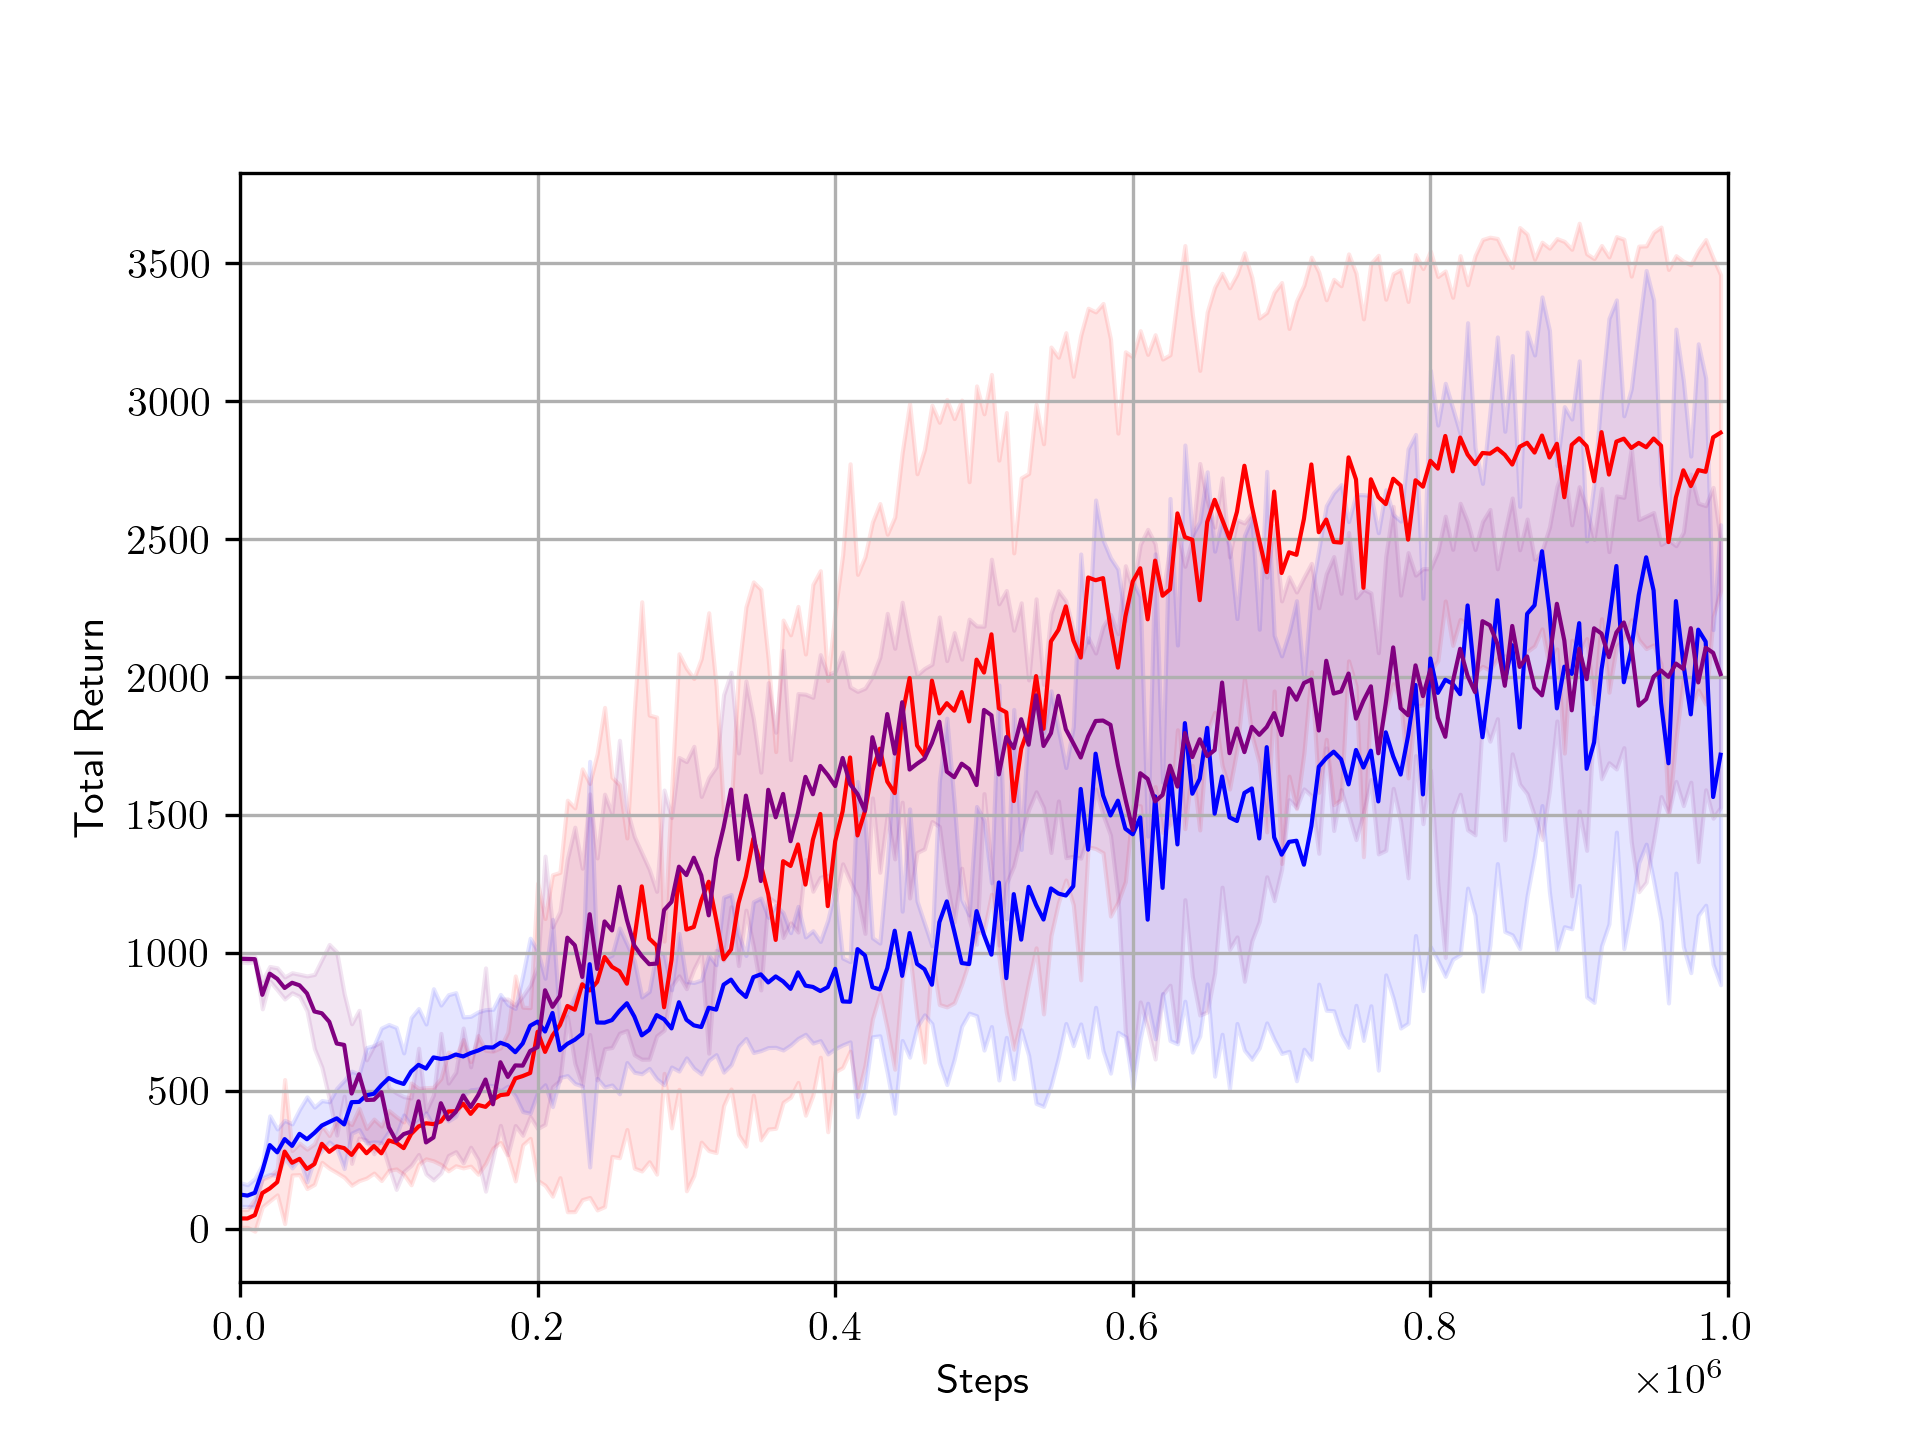}
    \caption{Hopper}
    % \label{fig:rvi_ablation}
  \end{subfigure}
  \begin{subfigure}{.3\textwidth}
    \centering
    \includegraphics[width=\linewidth]{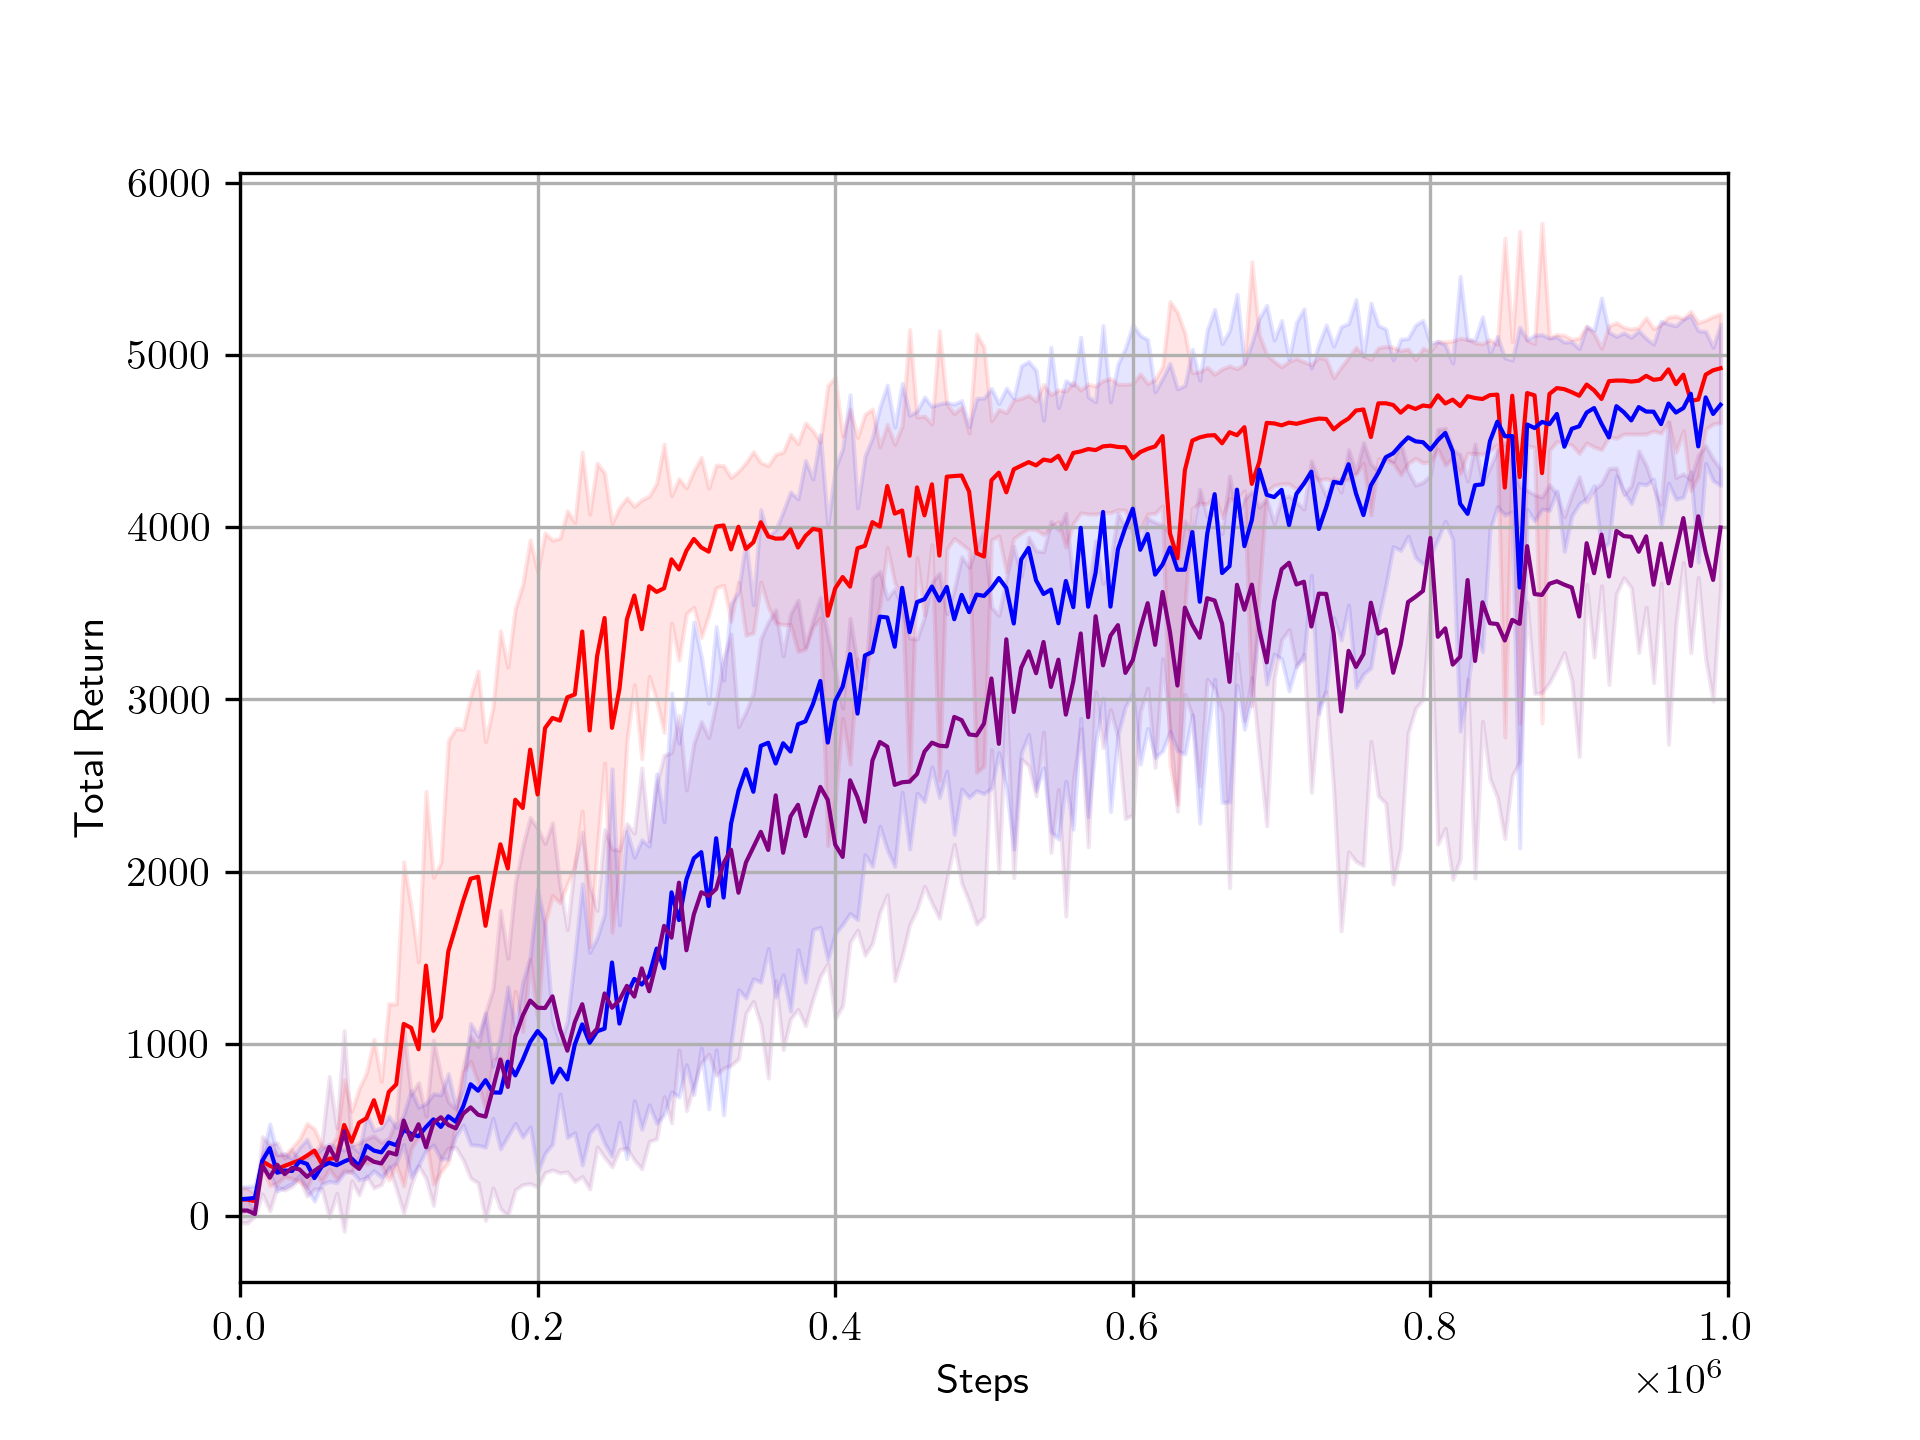}
    \caption{Walker2d}
    % \label{fig:fixed_reset}
  \end{subfigure}
  \begin{subfigure}{.3\textwidth}
    \centering
    \includegraphics[width=\linewidth]{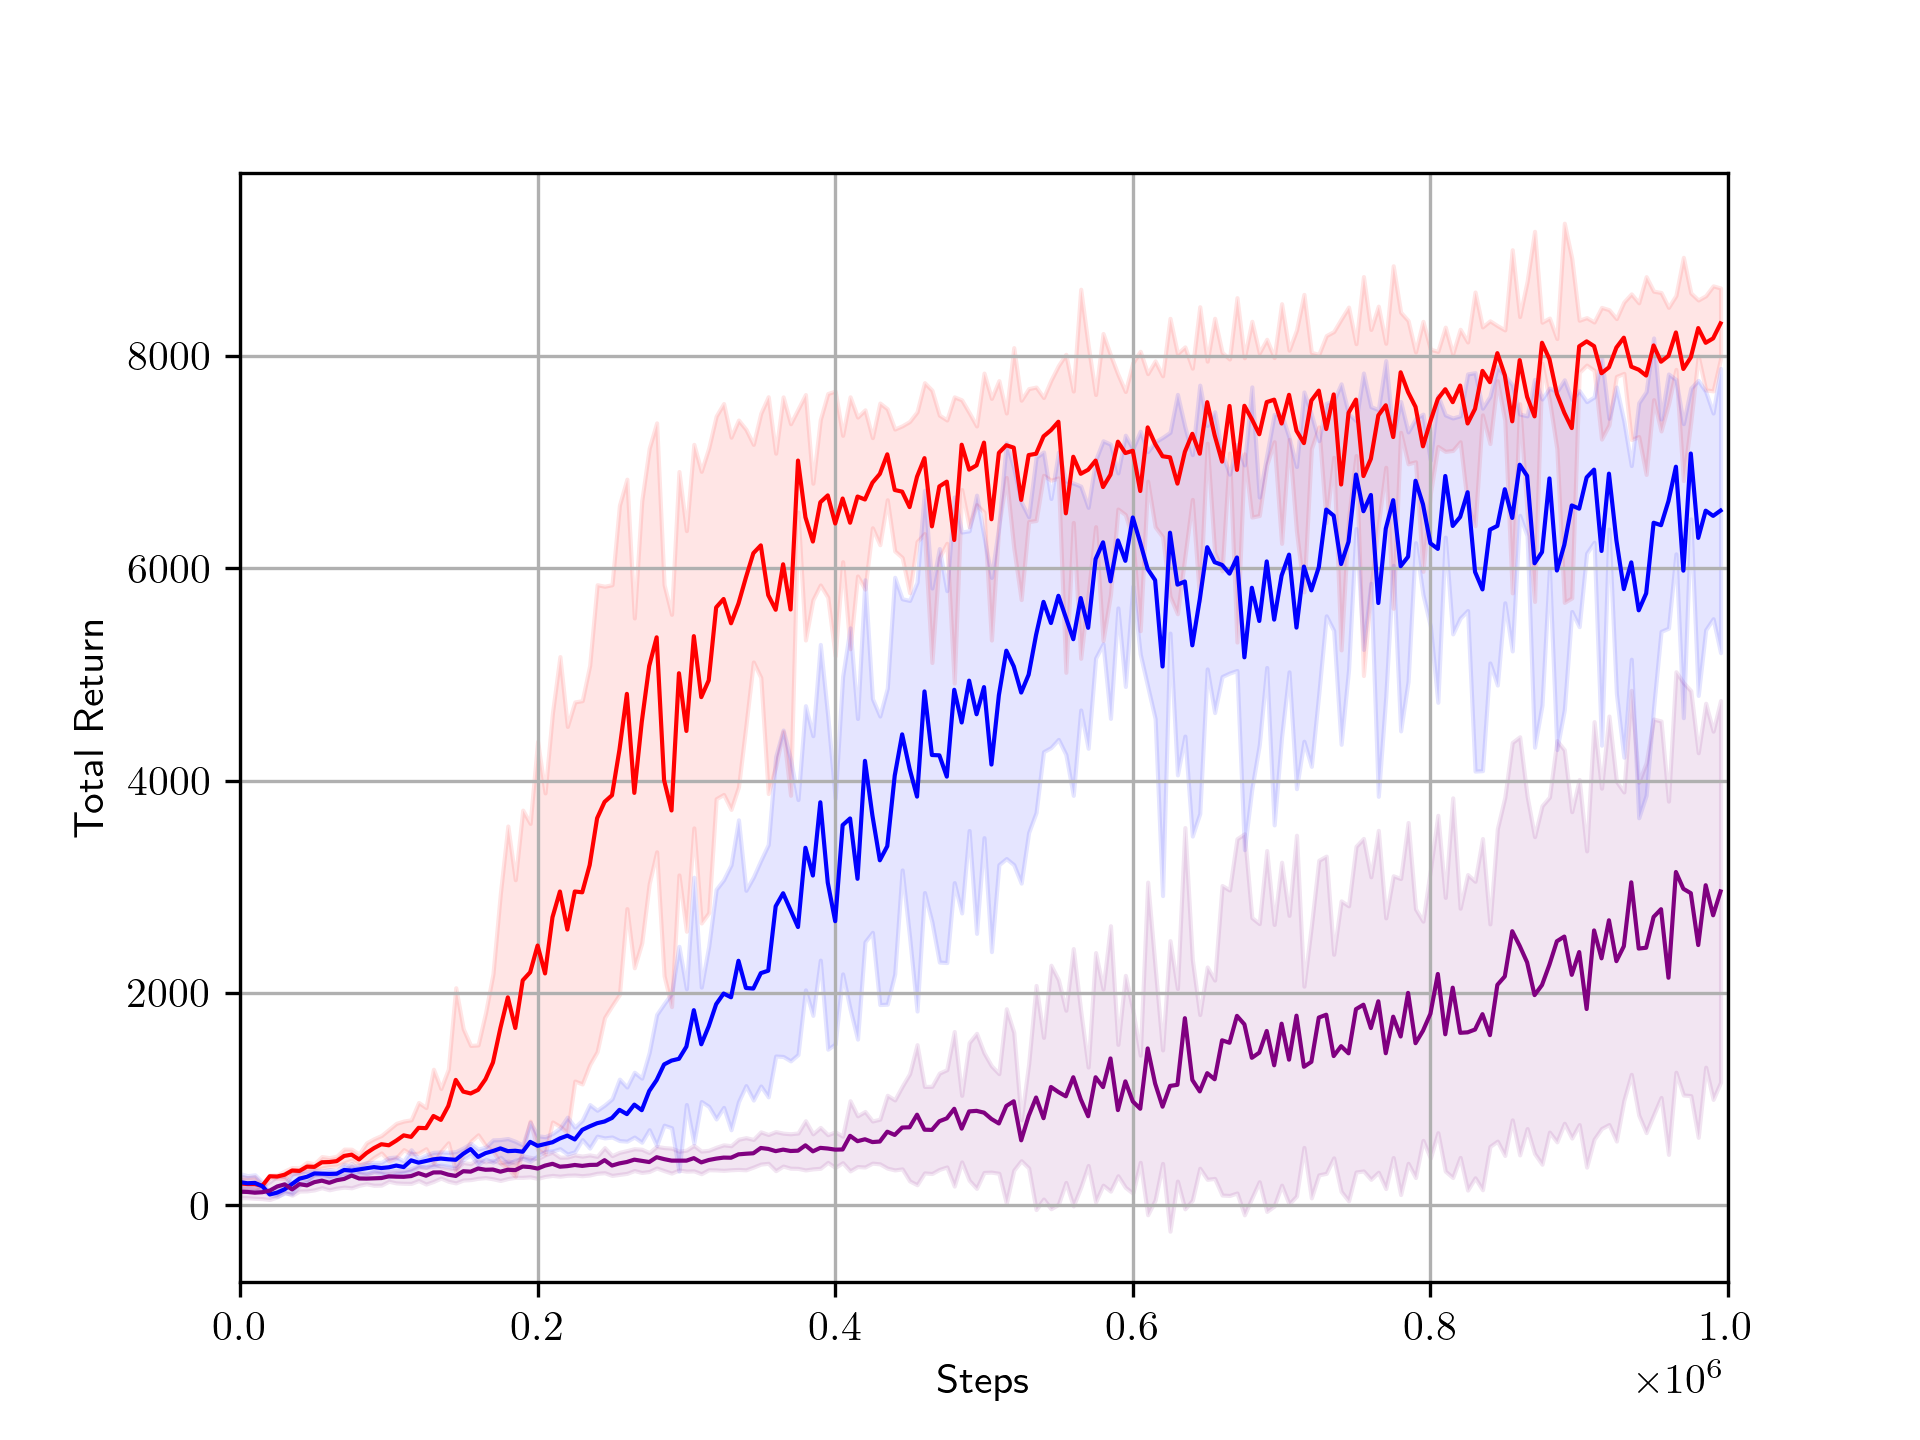}
    \caption{Humanoid}
    % \label{fig:fixed_reset}
  \end{subfigure}
  % \label{fig:average_reward}
  % \caption{Experimental results to show the effectiveness of each element of RVI-SAC. All three graphs are experimental results for the Ant environment.}
\end{figure*}
