# Supplementary material for: RVI-SAC: Average Reward Off-Policy Deep Reinforcement Learning
Source: arXiv:2408.01972 source file (2024-08-04)
Supplement: Supplementary file 4 [file experiment_delayed_fq_update.tex]

\section{\ref{sec:RVI_Q_learning_based_Q_Network_update}節に関する実験}

\begin{screen}
  Reference Stateを用いる方法は，連続な状態/行動空間を持つ問題にも容易に拡張可能であるが，Reference Stateへの訪問頻度やそのQ値の精度にアルゴリズム全体の性能が依存する懸念がある．\cite{Wan2020DifferentialQLearning}
\end{screen}
と述べたところに関する実験を行ったところ，提案手法の有効性を明確に述べられるような結果が得られなかった．

原理上，$f(Q)$の計算にReference Stateを用いる方法は，アルゴリズムが，そのReference Stateの選択に依存する．
その選択によって，性能が変わることはテーブル型の既存研究で指摘されている．\cite{Wan2020DifferentialQLearning}
しかし，mujoco環境では，その様子が観察されづらい．

以下の実験は，提案手法と，適当なReference State$(S,A)$を環境からサンプルし，
$$
f(Q_{\phi'}) = Q_{\phi'}(S,A)
$$
とした場合の性能を比較するものである．
\begin{figure}[H]
  \centering
  \includegraphics[width=0.5\linewidth]{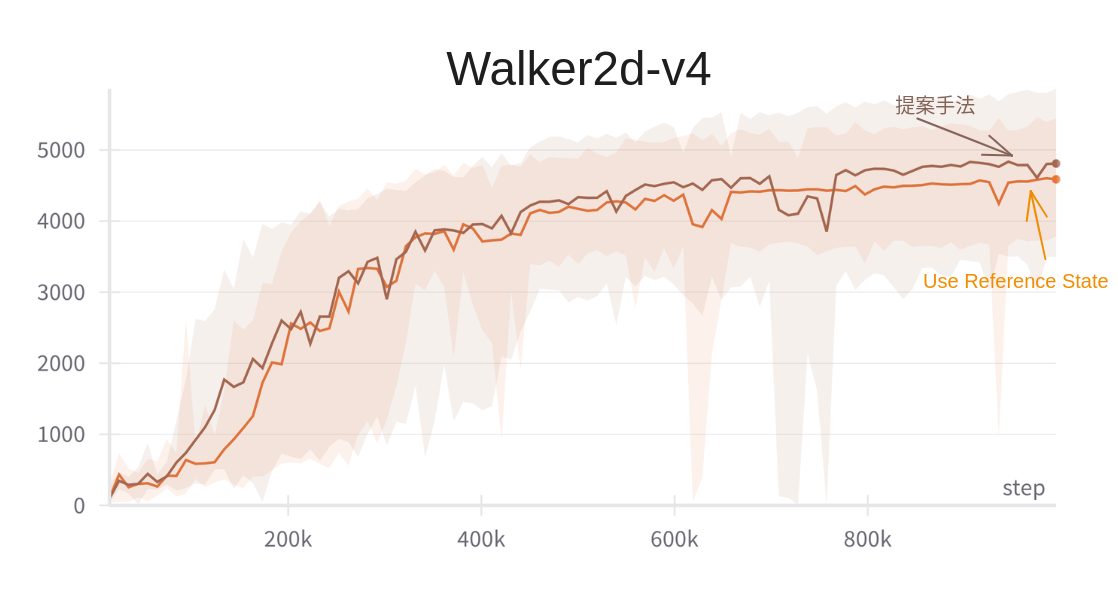}
  \label{fig:appendix:fig1}
\end{figure}
\begin{figure}[H]
  \centering
  \includegraphics[width=0.5\linewidth]{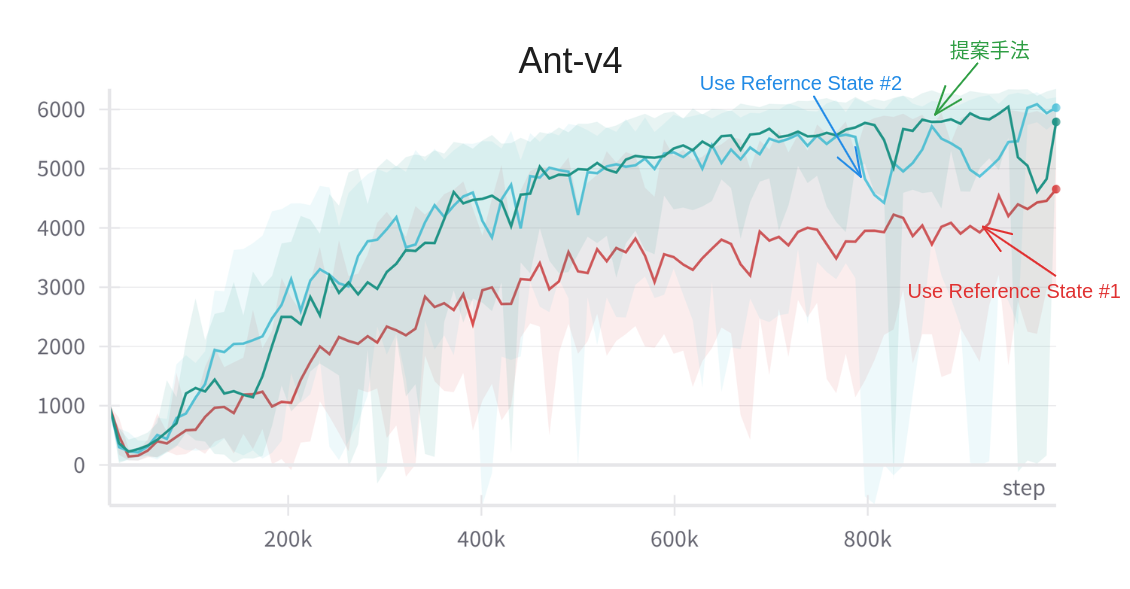}
  \label{fig:appendix:fig2}
\end{figure}

Use Reference Stateとしているものが，適当なReference Stateを用いて$f(Q_{\phi'}) = Q_{\phi'}(S,A)$としたものである．
上の実験結果では，AntとReference State\#1に対してのみ，理想的な結果を得られており，Walker2dでは得られなかった．
手元で実験を回している手応えとしては，SwimmerやHumanoidでもWalker2dと同様の結果が得られるとおもわれ，mujocoの全環境に対して，有効な実験が示せない．
mujocoで，このような結果が得られる原因としては，状態の各次元の要素の値の範囲が大きくて$-10 \sim 10$，小さくて$-1 \sim 1$の範囲に収まるように調整されていることが考えられる．
この値に調整されることにより，Reference Stateとして訪問頻度の低い状態を選択しても，その周りの状態のQ値が更新されることにより，Reference StateのQ値を調整することができるからである．

自分の主張においては，「Reference Stateに全体の性能が依存する懸念・可能性がある」ということなので，そのような現象が発生するAntのみでも主張は成り立たないことはない．
現状は，このAntのみ実験結果を用いて，上の主張を裏付けようと考えているが，より明確に主張を裏付ける別の方法を考えている．
\begin{itemize}
  \item 全環境において，性能が悪くなるようなReference Stateを見つけ出す．
  \item この問題がより明確に現れるような環境(mujoco以外)で実験する．
  \item 自分でToy Problemを作成する．
\end{itemize}
