# Supplementary material for: RVI-SAC: Average Reward Off-Policy Deep Reinforcement Learning
Source: arXiv:2408.01972 source file (2024-08-04)
Supplement: Supplementary file 5 [file hyperparameter.tex]

\section{Hyperparameter settings}
\label{sec:hyperparameter_settings}

\begin{table*}[H]
  \centering
  \begin{tabular}{lll}
    \toprule
                           & RVI-SAC & SAC                 \\
    \midrule
    Discount Factor        & N/A     & [0.99, 0.97, 0.999] \\
    Learning Rate          & 3e-4    & 3e-4                \\
    Batch Size             & 256     & 256                 \\
    Replay Buffer Size     & 1e6     & 1e6                 \\
    Target Update Interval & 1       & 1                   \\
    Offset Update TAU      & 1e-2    & N/A                 \\
    \bottomrule
  \end{tabular}
\end{table*}
